# Supplementary material for: Review of ultrasonic methods for monitoring, damage detection, and processing of lithium-ion batteries throughout their life-cycle
Source: arXiv:2601.08075 ancillary file (2026-06-15)
Supplement: Supplementary file 1 [file SupplementaryMaterialRevised.pdf]

## SUPPLEMENTARY MATERIAL FOR “REVIEW OF ULTRASONIC METHODS FOR MONITORING, DAMAGE DETECTION, AND PROCESSING OF LITHIUM-ION BATTERIES THROUGHOUT THEIR LIFE-CYCLE”

Simon Montoya-Bedoya, Tyler M. McGee, Joong Seok Lee, Sasha Litvinov, Ofodike A. Ezekoye, Donal P. Finegan, and Michael R. Haberman\*

This Supplemental Material (SM) provides an overview of the equations describing wave motion in elastic, viscoelastic, and poroelastic media. The derivations are focused on bulk waves in homogeneous elastic media, but also introduce the topic of Lamb waves propagating in isotropic elastic plates. More general descriptions of guided waves in anisotropic media or non-planar geometries are left for specialized literature. The topic of wave propagation in poroelastic media is also introduced via Biot’s theory. Finally, the SM provides practical information regarding the implementation of these models using transfer and stiffness matrix methods to predict wave propagation through multi-layered elastic and poroelastic media.

### S1. ELASTIC AND VISCOELASTIC MEDIA

The stress and strain in a medium that can be described by the linear elastodynamic wave equations are represented by the stress tensor  $\boldsymbol{\sigma}$  with components  $\sigma_{ij}$  and strain tensor  $\boldsymbol{\varepsilon}$  with components  $\varepsilon_{kl}$ . Note that some expressions in this section are written in both tensor and index form for the sake of clarity. The strain tensor is defined as the symmetric part of the displacement gradient  $\boldsymbol{\varepsilon} = (1/2) [\nabla \mathbf{u} + (\nabla \mathbf{u})^T] \leftrightarrow \varepsilon_{kl} = (1/2)(u_{k,l} + u_{l,k})$ , where  $\mathbf{u}$  is the displacement vector and a comma in the subscript denotes the spatial derivative. In linear elastic media, the stress and strain are related to each other through the generalized form of Hooke’s law<sup>1–3</sup>

$$\boldsymbol{\sigma} = \mathbf{C} : \boldsymbol{\varepsilon} \leftrightarrow \sigma_{ij} = C_{ijkl} \varepsilon_{kl}, \quad (1)$$

where  $\mathbf{C}$  is the fourth-order stiffness tensor and the  $:$  operator denotes the double inner product and we employ the Einstein summation convention on repeated indices. Note that the application of the elastic-viscoelastic correspondence principle allows one to represent the stiffness tensor as a complex quantity to capture phase delays between an applied strain and the resulting stress for time-harmonic wave motion<sup>2</sup>. Specifically, the viscoelastic stiffness tensor may be written as  $\mathbf{C} = \mathbf{C}' + j\mathbf{C}''$  where  $\mathbf{C}'$  is the elastic storage modulus and  $\mathbf{C}''$  is the loss modulus, which is zero when the medium is lossless. We can further note that the direction-dependent viscoelastic loss factor of any stiffness component,  $\eta_{ijkl}$ , is defined as the ratio of the loss and storage modulus of the component,  $\eta_{ijkl} = C''_{ijkl}/C'_{ijkl}$ .

The equations of motion in elastic media with the quiescent density  $\rho_0$  is given by

$$\nabla \cdot \boldsymbol{\sigma} = \rho_0 \frac{\partial^2 \mathbf{u}}{\partial t^2} \leftrightarrow \sigma_{il,l} = C_{ilmn} u_{m,n} = \rho \frac{\partial^2 u_i}{\partial t^2}, \quad (2)$$

where the displacement in Eq. (2) has a solution (using the  $e^{j\omega t}$  convention) in the form of  $\mathbf{u} = A \mathbf{p} e^{j(\omega t - \mathbf{k} \cdot \mathbf{x})}$  for time-harmonic plane waves of amplitude  $A$  propagating at a radian frequency  $\omega$  in the direction  $\mathbf{n}$ , a polarization vector  $\mathbf{p}$  denoting the direction of particle displacement, and with a wavenumber magnitude,  $k^2 = k_i k_i = k_1^2 + k_2^2 + k_3^2$ . Note that the components of the wavenumber are defined based on the phase velocity along the principle directions such that  $\mathbf{k} = \omega \mathbf{s}$ , where  $\mathbf{s}$  is the slowness vector with components  $s_i = v_i^{-1}$  and  $v_i$  being the phase velocity in the  $i^{\text{th}}$  direction.

Inserting the plane wave solution for the displacement into Eq. (2) yields the well-known Christoffel equation:<sup>2,3</sup>

$$[\boldsymbol{\Gamma} - \rho_0 v^2 \mathbf{I}] \mathbf{p} = \mathbf{0} \leftrightarrow (C_{ilmn} n_l n_n - \rho_0 v^2 \delta_{im}) p_m = 0, \quad (3)$$

where  $\boldsymbol{\Gamma}$  is a second-order tensor defined in terms of the stiffness tensor and components of the propagation direction vector:  $\Gamma_{il} = C_{ilmn} n_l n_n$  and  $\delta_{ij}$  is the Kronecker delta. The Christoffel equation in Eq. (3) is an eigenvalue problem where the eigenvalues yield the phase velocity  $v_i$  in principle directions, and the polarization vector is the eigenvector describing the displacement basis for the respective wave propagating at phase velocity  $v_i$ . For a given wave propagation direction, Eq. (3) is a cubic algebraic equation with respect to the phase speed  $v$ . By solving  $\det(\boldsymbol{\Gamma} - \rho_0 v^2 \mathbf{I}) = 0$  for nontrivial solution of Eq. (3), three distinct wave speeds  $v_{\text{I}}$ ,  $v_{\text{II}}$ ,  $v_{\text{III}}$  and corresponding principal polarization directions  $\mathbf{p}_{\text{I}}$ ,  $\mathbf{p}_{\text{II}}$ ,  $\mathbf{p}_{\text{III}}$  are obtained. Equation 3 can be rewritten in terms of the wave number and angular frequency as  $[k^2 \boldsymbol{\Gamma} - \rho_0 \omega^2 \mathbf{I}] \cdot \mathbf{p} = \mathbf{0}$  to obtain the dispersion relation between the wavenumber  $k$  and frequency  $\omega$  in bulk elastic media.

In isotropic elastic media, the stiffness tensor  $C_{ilmn}$  in Eq. (4) is expressed with only two independent properties, i.e., the Lamé parameters  $\lambda$  and  $\mu$ , the latter being the shear modulus of the medium. These two constants can be related to other elastic moduli such as the Young’s modulus, bulk modulus, and Poisson’s ratio using well-known relations<sup>2</sup>. For this isotropic case, the equation of motion in Eq. (2) simplifies to Navier’s equations of motion:

$$(\lambda + \mu) \nabla (\nabla \cdot \mathbf{u}) + \mu \nabla \times (\nabla \times \mathbf{u}) = \rho_0 \frac{\partial^2 \mathbf{u}}{\partial t^2}. \quad (4)$$

Since the wave propagation direction  $\mathbf{n}$  in isotropic elastic media is always either parallel or transverse to the displacement polarization direction  $\mathbf{p}$ , only purely longitudinal or shear waves will propagate with phase velocities  $c_l$  and  $c_s$ , respectively, which are related to the Lamé parameters through the relations:

$$c_l = v_{\text{I}} = \sqrt{\frac{\lambda + 2\mu}{\rho}}, \quad c_s = v_{\text{II}} = v_{\text{III}} = \sqrt{\frac{\mu}{\rho}}. \quad (5)$$

In anisotropic media, the polarization vectors cannot be identified as being purely longitudinal or transverse except when the wave propagation direction is specified

as the symmetry direction of the media. The propagation speeds  $v_{I,II,III}$  of three orthogonal waves from Eq. (3) correspond to one quasi-longitudinal wave and two quasi-vertical and horizontal shear waves.

In bounded media, propagating waves are dispersive (i.e. the phase speed is frequency-dependent) as a result of the interaction of the displacement field with domain boundaries, yielding a guided as illustrated in Fig. S1.B1 (this figure is repeated here from Fig. 2 of the manuscript for the convenience of the reader). The displacement field of guided waves in elastic plates are of specific interest to ultrasonic inspection and characterization of LIBs and are therefore briefly described here. These waves are an infinite set of propagating modes that are described by particle motion along the wave propagation direction ( $x$  direction) and the thickness direction ( $z$  direction). The guided wave modes, which are known as Lamb waves<sup>1</sup>, are solutions to Eq. 4 subject to traction-free boundary conditions at the “top” and “bottom” boundaries of the waveguide and they consist of an infinite set of symmetric (S) and antisymmetric (A) deformation modes as indicated in Figs. S1.B2-3. The wavenumber-frequency pairs for Lamb waves are found by solving for the roots of the characteristic equation provided in Eq. 6, where the wavenumber in question is the wavenumber along the  $x$  axis for the mode propagating at frequency  $\omega$ .<sup>1,3</sup>

$$\frac{\tan(\beta d/2)}{\tan(\alpha d/2)} + \left\{ \frac{4\alpha\beta k^2}{(\beta^2 - k^2)^2} \right\}^{\pm 1} = 0. \quad (6)$$

In this expression,  $\alpha^2 = \omega^2/c_t^2 - k^2$  and  $\beta^2 = \omega^2/c_s^2 - k^2$  where  $d$  is the plate thickness. The powers of +1 and -1 in Eq. (6) correspond to the relations for the symmetric and antisymmetric modes, respectively. From Eq. (6), the phase velocities  $c_{ph} = \omega/k$  and the group velocity  $c_g = \partial\omega/\partial k$  of each mode can be obtained for all frequencies. Note that the roots of this characteristic equation are known as the Rayleigh-Lamb spectrum and, contrary to the linear  $k$ - $\omega$  relation of bulk waves, the dispersion relation is nonlinear for Lamb waves.

## S2. POROELASTIC MATERIALS

Due to the microscopic structure and bi-phase composition between solid and fluid phases, ultrasonic waves propagating in poroelastic media experience severe attenuation in high frequencies and are strongly dispersive at low frequencies. The frequency range of interest in ultrasonic testing of LIBs is generally high, from hundreds of kHz to several MHz, while the thicknesses of layers within LIBs are on the order of tens of  $\mu\text{m}$ . In this sense, information about the dispersion relation and attenuation in single/multiple poroelastic layers is important for the use of ultrasonic waves in LIBs.

According to Biot's theory, the stress tensors of the solid and fluid phases,  $\sigma^s$  and  $\sigma^f$ , in isotropic and homogeneous porous media are described by the derivations of the solid and fluid phase displacements,  $\mathbf{u}$  and  $\mathbf{U}$ , re-

spectively, as:<sup>4,5</sup>

$$\sigma^s = A\nabla \cdot \mathbf{u}\mathbf{I} + 2N\varepsilon + Q\nabla \cdot \mathbf{U}\mathbf{I}, \quad (7a)$$

$$\sigma^f = Q\nabla \cdot \mathbf{u}\mathbf{I} + R\nabla \cdot \mathbf{U}\mathbf{I}, \quad (7b)$$

where  $\varepsilon$  denotes the strain tensor of the solid phase and  $\mathbf{I}$  is an identity tensor. The coefficients  $A$  and  $N$  are the Lamé constant and shear modulus, respectively. The variable  $Q$  is the coefficient accounting for the coupling effect by dilatational motions between the solid and fluid phases, and  $R$  is directly related to the bulk deformation of the fluid phase. These coefficients are intricately related to the elastic properties of the solid and fluid phases, such as the bulk modulus of the solid phase material made of ( $K_s$ ), the bulk modulus of the solid skeletal frame *in vacuo* ( $K_b$ ), and the bulk modulus of fluid phase ( $K_f$ ), with the porosity  $\phi$ .<sup>6,7</sup>

The equations of motion in poroelastic media are written as:<sup>4</sup>

$$N\nabla^2\mathbf{u} + \nabla[(A+N)\nabla \cdot \mathbf{u} + Q\nabla \cdot \mathbf{U}] = \rho_{11}\frac{\partial^2\mathbf{u}}{\partial t^2} + \rho_{12}\frac{\partial^2\mathbf{U}}{\partial t^2} + b\left(\frac{\partial\mathbf{u}}{\partial t} - \frac{\partial\mathbf{U}}{\partial t}\right) \quad (8)$$

$$\nabla[Q\nabla \cdot \mathbf{u} + R\nabla \cdot \mathbf{U}] = \rho_{12}\frac{\partial^2\mathbf{u}}{\partial t^2} + \rho_{22}\frac{\partial^2\mathbf{U}}{\partial t^2} + b\left(\frac{\partial\mathbf{U}}{\partial t} - \frac{\partial\mathbf{u}}{\partial t}\right), \quad (9)$$

where the left-hand sides of Eqs. (8) and (9) correspond to  $\nabla \cdot \sigma^s$  and  $\nabla \cdot \sigma^f$ , respectively. The effective density of poroelastic media  $\rho_{11}$ ,  $\rho_{12}$ , and  $\rho_{22}$  account for the effects of momentum transfer between the solid and fluid phases resulting from the porosity  $\phi$  and tortuosity  $\alpha_\infty$ . They are defined as  $\rho_{11} = \rho_1 + \rho_a$ ,  $\rho_{22} = \rho_2 + \rho_a$ , and  $\rho_{12} = -\rho_a$  with  $\rho_1 = (1-\phi)\rho_s$ ,  $\rho_2 = \phi\rho_f$ ,  $\rho_a = (\alpha_\infty - 1)\phi\rho_f$ , where  $\rho_s$  and  $\rho_f$  denote the densities of the solid and fluid phases, respectively. In Eqs. (8),(9),  $b$  is a frequency-dependent and complex-valued quantity accounting for the viscous coupling between two phases. Under the time harmonic motion, the effective densities can be rewritten to include the viscous coupling effect as  $\rho_{11}^* = \rho_{11} + b/j\omega$ ,  $\rho_{12}^* = \rho_{12} - b/j\omega$ , and  $\rho_{22}^* = \rho_{22} + b/j\omega$ .

The equations of motion of Eqs. (8) and (9) can be decomposed into two scalar Helmholtz equations governing two longitudinal and one shear wave, respectively, by conducting the standard Helmholtz decomposition to the solid and fluid phase displacement vectors in Eqs. (8) and (9). From the scalar Helmholtz equations, the wavenumbers propagating in poroelastic media are found to be:<sup>7,8</sup>

$$k_{1,2}^2 = \omega^2 \frac{(P\rho_{22}^* + R\rho_{11}^* - 2Q\rho_{12}^*) \pm \sqrt{\Delta}}{2(PR - Q^2)}, \quad (10a)$$

$$k_3^2 = \omega^2 \frac{\rho_{11}^* - \rho_{12}^*/\rho_{22}^*}{N}, \quad (10b)$$

where  $k_{1,2}$  denote the wavenumbers of two longitudinal modes and  $k_3$  is the shear wavenumber with  $P = A + 2N$

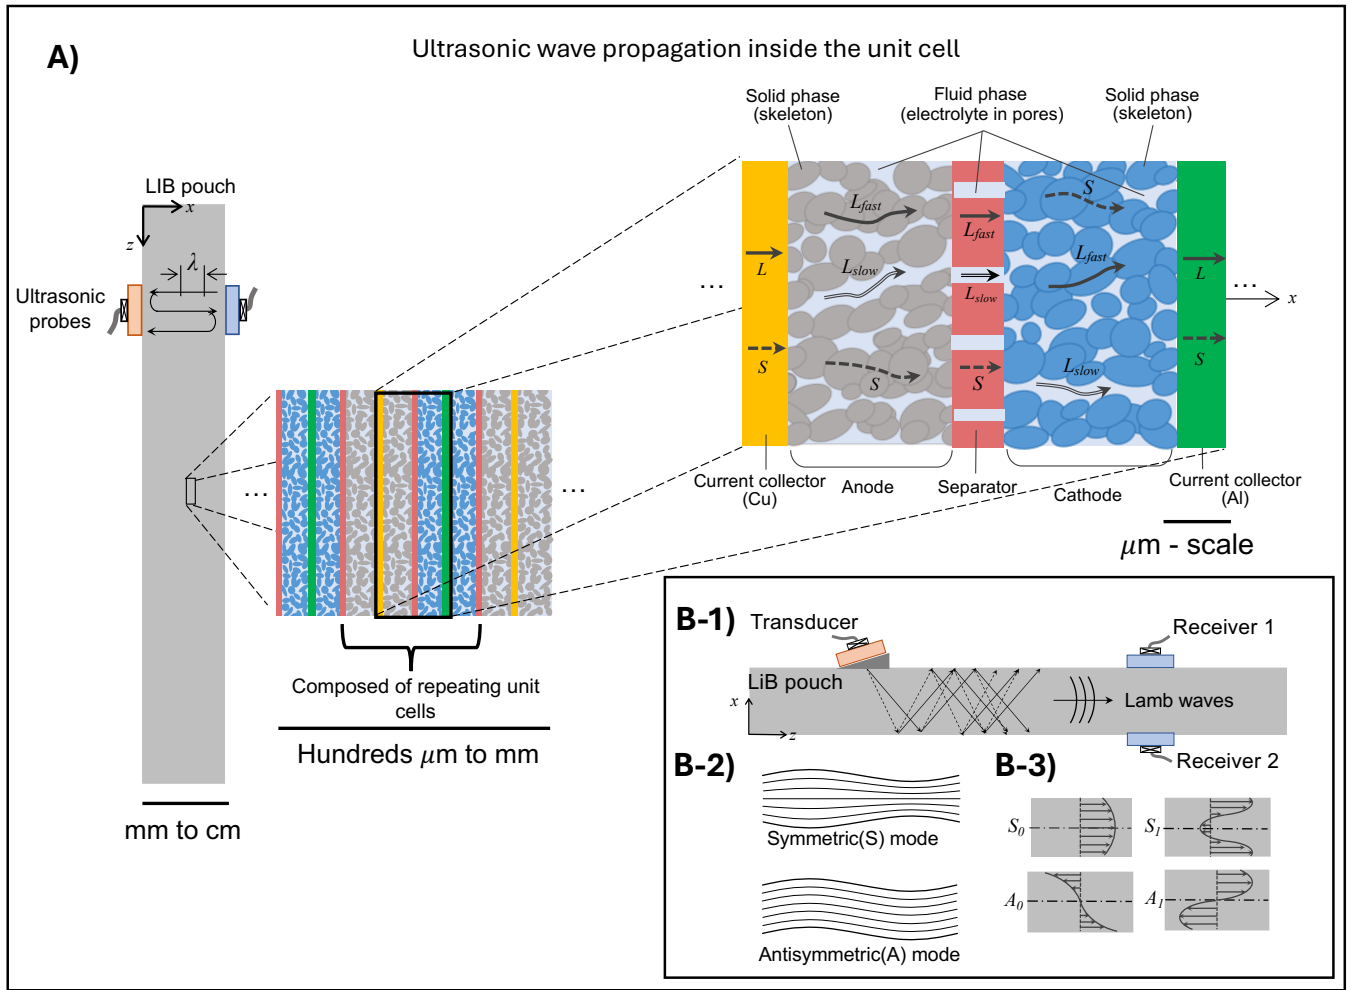

FIG. S1. **(A)** Schematic of ultrasonic wave propagation through a LIB pouch cell, highlighting the layered structure composed of repeating unit cells, which include current collectors (Cu and Al), anode, separator, and cathode. For the porous materials, each layer consists of a solid skeleton and fluid-filled pores (electrolyte). Longitudinal (L) and shear (S) waves propagate through the solids, while only longitudinal waves propagate through the fluid phase. Scale bars are not exact. They are provided as a generic reference scale for microscale (0.5–100  $\mu\text{m}$ ) and macroscale (> 0.1 mm) features. **(B)** Scheme of guided wave generation and detection using ultrasonic probes: (B-1) Experimental setup showing guided wave propagation along the  $z$ -direction. (B-2) Illustration of symmetric (S) and antisymmetric (A) Lamb wave modes in the LIB pouch. (B-3) Various modes of Lamb waves ( $S_0$ ,  $S_1$ ,  $A_0$ ,  $A_1$ ) and their relative particle displacement profiles across the thickness of the pouch.

and  $\Delta = (P\rho_{22}^* + R\rho_{11}^* - 2Q\rho_{12}^*)^2 - 4(PR - Q^2)(\rho_{11}^*\rho_{22}^* - \rho_{12}^{*2})$ . From Eq. (10), the phase velocities and attenuation coefficients (imaginary part of the wavenumber) of the three waves propagating in poroelastic media are calculated by  $c_{\text{ph},i} = \omega/\text{Re}\{k_i\}$  and  $\alpha_i = -\text{Im}\{k_i\}$ , respectively ( $i = 1, 2, 3$ ), and we note that the comma in the subscript of the phase velocity designates the index and does not denote the spatial derivative.

As illustrated in Fig. S1, the existence of three kinds of propagating waves in a poroelastic material is distinguishable from the two bulk wave modes (one longitudinal wave and one shear wave) propagating in an isotropic elastic medium. By comparing their phase velocities, two longitudinal waves in a poroelastic material are classified

as the *fast* and *slow* waves. The conventional interpretation of these waves is that the fast wave (sometimes called the frame-borne wave) is primarily borne in the stiffer elastic frame (i.e. the “solid phase”), while the slow wave (or the fluid-borne wave) propagates mainly in the interstitial fluid within the pores of the poroelastic material. However, we note that this explanation is an oversimplification because both longitudinal modes result from coupling between the solid and fluid phases where the majority of the energy in the fast wave is carried in the elastic frame and the converse is true for the slow wave. In addition, according to Biot’s original work<sup>4</sup>, the particle motion of the solid and fluid phases are in phase in the fast wave, while the displacements of the two phases

are out-of-phase for the slow wave. It is for this reason that the slow wave has significantly higher attenuation during propagation than the fast wave.

Theoretical descriptions for poroelastic material modeling based on Biot's theory for electrodes or separators in LIBs can be found in Refs.<sup>9–14</sup>, but those works did not expand the interpretation of the physical phenomena of poroelasticity as it pertains to LIBs beyond general descriptions in Biot's original<sup>4,5</sup> and generalized works<sup>15,16</sup>. Together with the coupled governing equations, the generalized elasticity coefficients ( $A$ ,  $N$ ,  $Q$ ,  $R$ ) and effective dynamic densities ( $\rho_{11}^*$ ,  $\rho_{12}^*$ ,  $\rho_{12}^*$ ) appearing in the equations should properly account for the intricate coupling effects during wave propagation and attenuation in poroelastic media. Regarding the attenuation of acoustic energy, the viscous, inertial, and thermal energy conversion due to relative motion between solid and fluid phases in poroelastic materials results in frequency-dependent, complex elasticity coefficients and effective densities<sup>6,17,18</sup>. One common application of porous media is noise reduction applications that employ foams, which are air-saturated, sound-absorbing poroelastic materials, where the dissipation caused by all three kinds of coupling effects is critical to improve performance. However, LIB-related literature that employs poroelastic material modeling tends to simplify the coupling effects. Namely, dissipation by viscous effect has been accounted for in the complex quantity  $b$  in the generalized complex densities  $\rho_{11}^*$ ,  $\rho_{12}^*$ , and  $\rho_{12}^*$ , but inertial coupling was partly omitted with assumptions<sup>10,11,13</sup> and to date the LIB literature that employs poroelastic modeling has not considered thermal dissipation effects, resulting in real-valued generalized elasticity coefficients in the governing equations. Such simplifications may be allowable in the poroelastic material modeling in LIBs because the porosities in the electrodes and separators in LIBs are remarkably low when compared to typical values in sound-absorbing poroelastic materials. Specifically, given the fact that the typical value of the bulk modulus of the electrolytes in LIBs (i.e. the fluid phase in electrodes and separators) is on the same order of magnitude as that of water ( $\sim 10^9$  Pa)<sup>19</sup>, the use of real-valued generalized coefficients  $Q$  and  $R$  may be realistic when modeling waves in LIBs, as is the case for many geophysical applications.

One additional metric that is relevant to the modeling of ultrasonic waves in LIBs is Biot's characteristic frequency, which provides a demarcation between frequency regimes where inertial or viscous effects dominate in poroelastic materials. This frequency is defined by the relation  $f_c = \eta\phi/(2\pi\alpha_\infty\rho_f q_0)$  where  $\eta$  is the dynamic fluid viscosity and  $q_0$  represents the static permeability. Viscous effects are dominant in the frequency regions below  $f_c$ , while the inertial effect becomes more apparent above  $f_c$ . According to Gor et al.<sup>19</sup>, typical values of the static permeability of graphite anode and the fluid viscosity of electrolytes in LIBs are 0.04 darcy and 0.042 Pa·s, respectively. These values were used in the poroelastic material modeling in LIB in Refs.<sup>9–11,13</sup>. Given the fact that the fluid densities of electrolytes are close to that of

water, these properties result in  $f_c$  ranging from hundreds of kHz to tens of MHz. This implies that viscous effects and concomitant strong attenuation will be present for most ultrasonic wave propagation in LIBs.

### S3. MODEL IMPLEMENTATION

In modeling poroelastic material layers using the transfer matrix method, six state variables are required to represent wave motion, resulting in  $6 \times 6$  transfer matrix for a poroelastic layer.<sup>8,20–22</sup> The state variable vector can be chosen to be different combinations of variables, for example,  $\{u_n, u_s, U_n, \sigma_n^s, \sigma_{ns}^s, \sigma^f\}$ <sup>7,8</sup>,  $\{u_n, u_s, \phi(U_n - u_n), \sigma_n^t, \sigma_{ns}^s, p\}$ <sup>20</sup>,  $\{u_n, u_s, u_n^t, \hat{\sigma}_n^s, \hat{\sigma}_{ns}^s, p\}$ <sup>22,23</sup>, etc., where the subscripts  $n$ ,  $s$ ,  $ns$  denote the normal, tangential, and shear components of the variables, respectively, and  $p$ ,  $\sigma^t$ , and  $\hat{\sigma}^s$  are the interstitial pressure in pores, the total stress, and the stress of the solid phase *in vacuo*, respectively. To account for multiple poroelastic layers in LIBs, such as anodes/cathodes and electrodes having dissimilar properties, the displacement continuities and force equilibrium should be satisfied along interfaces between dissimilar poroelastic layers<sup>24,25</sup>. To model a multilayered LIB cell, elastic layers in the electrodes and interface couplings between elastic and poroelastic layers should be considered as well. Since the transfer matrix of an elastic layer ( $4 \times 4$ ), which is a different order than that of a poroelastic layer ( $6 \times 6$ ), the interface coupling matrices between them are not square, and therefore the transfer matrices for different types of media (poroelastic and elastic) cannot be directly multiplied to build a sort of a global transfer matrix. Rather, one must build a global matrix by assembling the individual transfer matrices and interface coupling matrices<sup>7</sup>.

Compared with the transfer matrix method, the stiffness matrix method builds the displacement-force relation in a layer by defining a stiffness matrix<sup>11,26,27</sup>. Since the stiffness matrix equation is individually defined at each layer, stiffness matrices for individual layers and their interface coupling matrices should be assembled into a global matrix to represent multilayered LIBs. Although a recursive algorithm can reduce the global matrix size for stiffness matrices of a similar nature, the assembly of a global matrix is unavoidable. According to previous works<sup>11,26,27</sup>, the stiffness matrix method is more stable than the transfer matrix approach, especially when calculating wave motion in high-frequency ranges. To get a dispersion relation of a periodic poroelastic multiple layers in LIBs, the Floquet-Bloch periodic boundary condition<sup>28</sup> can be imposed on the global matrix of the unit cell of the periodic medium. Since the global matrix is formed by assembly of many transfer (or stiffness) matrices of different nature, the imposition of periodic conditions does not yield a standard-form eigenvalue problem, which is obtained for periodic multilayers consisting of the same type. Instead, the Bloch wavenumbers satisfying zero determinant of the global matrix should be searched over the considered frequency range numeri-

cally. In general, the results of the root finding operation may depend on the implemented algorithm and contain many local optima, possibly causing spurious or missing branches in the dispersion curves. At the time of this writing, the complication encountered during implementation is inevitable because one must use the assembled global matrix to model waves propagating through multilayered media with different constitutive behaviors. We also note that both transfer and stiffness matrix approaches may have additional numerical complications associated with both (i) the fact that many layers are very thin compared to acoustic wavelengths, and (ii) at the high frequency range of interest where one may have multiple wavelengths within a single layer.

- <sup>1</sup>J. D. Achenbach, *Wave propagation in elastic solids*. Amsterdam: Elsevier Science Publishers, 1975.
- <sup>2</sup>R. M. Christensen, *Mechanics of Composite Materials*. Courier Corporation, 2012.
- <sup>3</sup>J. L. Rose, *Ultrasonic waves in solid media*. Cambridge University Press, 2004.
- <sup>4</sup>M. A. Biot, "Theory of Propagation of Elastic Waves in a Fluid-Saturated Porous Solid. I. Low-Frequency Range," *The Journal of the Acoustical Society of America*, vol. 28, no. 2, pp. 168–178, 1956.
- <sup>5</sup>M. A. Biot, "Theory of Propagation of Elastic Waves in a Fluid-Saturated Porous Solid. I. Low-Frequency Range," *The Journal of the Acoustical Society of America*, vol. 28, no. 2, pp. 168–178, 1956.
- <sup>6</sup>M. A. Biot and D. G. Willis, "The Elastic Coefficients of the Theory of Consolidation," *Journal of Applied Mechanics*, vol. 24, no. 4, pp. 594–601, 1957.
- <sup>7</sup>J. F. Allard and N. Atalla, *Propagation of Sound in Porous Media: Modelling Sound Absorbing Materials*. John Wiley & Sons, Ltd, 2nd ed., 2009.
- <sup>8</sup>J. Bolton, N.-M. Shiau, and Y. Kang, "Sound transmission through multi-panel structures lined with elastic porous materials," *Journal of Sound and Vibration*, vol. 191, no. 3, pp. 317–347, 1996.
- <sup>9</sup>L. Gold, T. Bach, W. Virsik, A. Schmitt, J. Müller, T. E. Staab, and G. Sextl, "Probing lithium-ion batteries' state-of-charge using ultrasonic transmission-concept and laboratory testing," *Journal of Power Sources*, vol. 343, pp. 536–544, 2017.
- <sup>10</sup>G. Jie, L. Yan, Z. Mingfang, L. Mingkun, L. Hongye, W. Bin, and H. Cunfu, "Guided waves propagation in multi-layered porous materials by the global matrix method and biot theory," *Applied Acoustics*, vol. 184, p. 108356, 2021.
- <sup>11</sup>M. Huang, F. Cegla, and B. Lan, "Stiffness matrix method for modelling wave propagation in arbitrary multilayers," *International Journal of Engineering Science*, vol. 190, p. 103888, 2023.
- <sup>12</sup>B. Zhang, Y. Lyu, J. Gao, G. Song, Y. chun Lee, C. He, W. Song, and H. Chen, "Ultrasonic reflection/transmission characteristics for state of charge of li-ion battery," *Applied Acoustics*, vol. 214, p. 109687, 2023.
- <sup>13</sup>G. Jie, Z. Liangheng, L. Yan, S. Fan, W. Bin, and H. Cunfu, "Ultrasonic guided wave measurement and modeling analysis of the state of charge for lithium-ion battery," *Journal of Energy Storage*, vol. 72, p. 108384, 2023.
- <sup>14</sup>S. Zhang, P. Zuo, X. Yin, and Z. Fan, "Exploring the correlation between ultrasound time of flight and the state of health of lifepo4 prismatic cells," *Journal of Energy Storage*, vol. 83, p. 110715, 2024.
- <sup>15</sup>M. A. Biot, "Generalized Theory of Acoustic Propagation in Porous Dissipative Media," *The Journal of the Acoustical Society of America*, vol. 34, no. 9A, pp. 1254–1264, 1962.
- <sup>16</sup>M. A. Biot, "Mechanics of Deformation and Acoustic Propagation in Porous Media," *Journal of Applied Physics*, vol. 33, no. 4, pp. 1482–1498, 1962.
- <sup>17</sup>D. L. Johnson, J. Koplik, and R. Dashen, "Theory of dynamic permeability and tortuosity in fluid-saturated porous media," *Journal of Fluid Mechanics*, vol. 176, p. 379–402, 1987.
- <sup>18</sup>Y. Champoux and J. Allard, "Dynamic tortuosity and bulk modulus in air-saturated porous media," *Journal of Applied Physics*, vol. 70, no. 4, pp. 1975–1979, 1991.
- <sup>19</sup>G. Y. Gor, J. Cannarella, J. H. Prévost, and C. B. Arnold, "A model for the behavior of battery separators in compression at different strain/charge rates," *Journal of The Electrochemical Society*, vol. 161, no. 11, p. F3065, 2014.
- <sup>20</sup>G. E. Baird, P. D. Thomas, and G. Sang, "The propagation of elastic waves through a layered poroelastic medium," *The Journal of the Acoustical Society of America*, vol. 99, no. 6, pp. 3385–3392, 1996.
- <sup>21</sup>A. K. Vashishth and P. Khurana, "Waves in stratified anisotropic poroelastic media: a transfer matrix approach," *Journal of Sound and Vibration*, vol. 277, no. 1, pp. 239–275, 2004.
- <sup>22</sup>O. Dazel, J.-P. Groby, B. Brouard, and C. Potel, "A stable method to model the acoustic response of multilayered structures," *Journal of Applied Physics*, vol. 113, no. 8, p. 083506, 2013.
- <sup>23</sup>J. S. Lee, "A new unified modeling of acoustically-coupled multilayers by  $(u^s, u^W)$  displacement formulation based poroelastic transfer matrix," *Journal of Mechanical Science and Technology*, vol. 29, no. 2, pp. 663–676, 2015.
- <sup>24</sup>H. Deresiewicz and R. Skalak, "On uniqueness in dynamic poroelasticity," *Bulletin of the Seismological Society of America*, vol. 53, no. 4, pp. 783–788, 1963.
- <sup>25</sup>O. M. Lovera, "Boundary conditions for a fluid-saturated porous solid," *Geophysics*, vol. 52, no. 2, pp. 174–178, 1987.
- <sup>26</sup>L. Wang and S. Rokhlin, "Stable reformulation of transfer matrix method for wave propagation in layered anisotropic media," *Ultrasonics*, vol. 39, no. 6, pp. 413–424, 2001.
- <sup>27</sup>S. I. Rokhlin and L. Wang, "Stable recursive algorithm for elastic wave propagation in layered anisotropic media: Stiffness matrix method," *The Journal of the Acoustical Society of America*, vol. 112, no. 3, pp. 822–834, 2002.
- <sup>28</sup>L. Brillouin, *Wave propagation in periodic structures*. Dover Publications, 1953.
